# Supplementary material for: AntLM: Bridging Causal and Masked Language Models
Source: arXiv:2412.03275 source file (2024-12-04)
Supplement: Supplementary file 1 [file 8_appendix.tex]

% \section{Example Appendix}
% \label{sec:appendix}

% This is an appendix.
